# Supplementary material for: Toward the Combinatorial Limit Theory of Free Words
Source: arXiv:1509.04372 source file (2015-09-15)
Supplement: Supplementary file 1 [file AppendixMD.tex]

%%%%%%%%%%%%%%%%%%%%%%%%%%%%%%%%%%%%%%%%%%%%
%\section{Summary of Results from Density.tex}
%%%%%%%%%%%%%%%%%%%%%%%%%%%%%%%%%%%%%%%%%%%%

\chapter{Summary of Bounds on Asymptotic Zimin Probabilities} \label{appendMD}

The following tables give numerical approximations for upper and lower bounds of $\underline{\delta}(Z_n,q)$ for various $n,q \geq 2$ as found in this manuscript.

%Lower/Upper (i.e., tight) bound from Theorem \ref{dZ2}:
\begin{table}[ht]
\centering
\begin{threeparttable}

	\caption{Tight bound for $n=2$ from Theorem \ref{dZ2}.}
%	\caption{Tight bound for $\underline{d} (Z_2,q)$ from Theorem \ref{dZ2}.}

	\begin{tabular}{c}
	$\begin{array}{c|c|c|c|c|c|c}
		&q&2&3&4&5&\cdots \\ \hline
		n = 2&\frac{1}{q}&.5&.333&.25&.2&\cdots
	\end{array}$
	\end{tabular}

\end{threeparttable}
\end{table}

%Lower bound from Theorem \ref{dZn} using $f(2,q)=2q+1$ and $f(3,2) = 29$:
\begin{table}[ht]
\centering
\begin{threeparttable}

	\caption{Lower bounds from Theorem \ref{dZn}.}
%	\caption{Lower bounds for $\underline{\delta}(Z_n,q)$ from Theorem \ref{dZn}.}

	\begin{tabular}{c}
	$\begin{array}{c|c|c|c|c|c|c}
		&q&2&3&4&5&\cdots \\ \hline
		n&\displaystyle\frac{1}{f(n-1,q)^2 q^{f(n-1,q)+1}}&&&&& \\ \hline
		3&& 6.25\cdot 10^{-4}& 3.11\cdot 10^{-6}& 1.18\cdot 10^{-8}& 3.39\cdot 10^{-11}&\cdots\\ \hline
		4 && 1.11\cdot 10^{-12} &&&&
	\end{array}$
	\end{tabular}

	\begin{tablenotes}[flushleft]
	\item Use $f(2,q)=2q+1$ for $n=3$ and $f(3,2) = 29$ for $n=4$.
	\end{tablenotes}

\end{threeparttable}
\end{table}

%Lower bound from Theorem \ref{dZn} using $f(3,q)\leq (2q+1)^{(2q+1)}$:
\begin{table}[ht]
\centering
\begin{threeparttable}

	\caption{Lower bounds for $n=4$ from Theorem \ref{dZn} using $f(3,q)\leq (2q+1)^{(2q+1)}$}
%	\caption{Lower bounds for $\underline{\delta}(Z_4,q)$ from Theorem \ref{dZn} using $f(3,q)\leq (2q+1)^{(2q+1)}$}

	\begin{tabular}{c}
	$\begin{array}{c|c|c|c|c|c}
		&q=2&3&4&q>4 \\ \hline
		n = 4& 9.78\cdot 10^{-949}& 6.64\cdot 10^{-392943}& 9.42\cdot 10^{-233250395}&SageRuntimeError
	\end{array}$
	\end{tabular}

\end{threeparttable}
\end{table}

%Lower bounds from Corollary \ref{dZ3}:
\begin{table}[ht]
\centering
\begin{threeparttable}

	\caption{Lower bounds for $n=3$ from Corollary \ref{dZ3}}
%	\caption{Lower bounds for $\underline{\delta}(Z_3,q)$ from Corollary \ref{dZ3}}

	\begin{tabular}{c}
	$\begin{array}{c|c}
		&q=2 \\ \hline
		n = 3& 1/54 \approx 1.85\cdot 10^{-2}
	\end{array}$\\

	$\begin{array}{c|c|c|c|c|c}
		&q&3&4&5&\cdots \\ \hline
		n = 3& 1/((2q-1)^2q!2^q)& 8.33\cdot 10^{-4} & 5.31 \cdot 10^{-5} & 3.22 \cdot 10^{-7} & \cdots
	\end{array}$
	\end{tabular}

\end{threeparttable}
\end{table}

%Upper bound from Section \ref{prob}:
\begin{table}[ht]
\centering
\begin{threeparttable}

	\caption{Upper bounds from Section \ref{prob}}
%	\caption{Upper bounds for $\underline{\delta}(Z_n,q)$ from Section \ref{prob}}

	\begin{tabular}{c}
	$\begin{array}{c|c|c|c|c|c}
		&q = 2&3&4&5&\cdots \\ \hline
		n = 2&  .732&.443 & .312 & .240 & \cdots\\ \hline
		3&  .119&1.84 \cdot 10^{-2} & 5.19 \cdot 10^{-3}& 2.00 \cdot 10^{-3} & \cdots
	\end{array}$
	\end{tabular}

\end{threeparttable}
\end{table}

%Upper bound from Section \ref{DeB}
\begin{table}[ht]
\centering
\begin{threeparttable}

	\caption{Upper bound for $n=3,q=2$ from Section \ref{DeB}}
%	\caption{Upper bound for $\underline{\delta}(Z_3,2)$ from Section \ref{DeB}}

	\begin{tabular}{c}
	$\begin{array}{c|c}
		&q=2 \\ \hline
		n = 3& 1/28 \approx 3.57\cdot 10^{-2}
	\end{array}$
	\end{tabular}

\end{threeparttable}
\end{table}

%Upper bound from Section \ref{nested}:
\begin{table}[ht]
\centering
\begin{threeparttable}

	\caption{Upper bounds from Section \ref{IV}}
%	\caption{Upper bounds for $\underline{\delta}(Z_n,q)$ from Section \ref{nested}}

	\begin{tabular}{c}
	$\begin{array}{c|c|c|c|c|c|c}
		&q&2&3&4&5&\cdots \\ \hline
		n&\displaystyle \prod_{\lambda = 1}^{n-1}\frac{1}{(q^{(2^\lambda - 1)} - 1)} &&&&\\ \hline
		3&  &.143&1.92\cdot10^{-2} & 5.29\cdot10^{-3} & 2.02\cdot10^{-3} & \cdots\\ \hline
		4&  &1.12\cdot10^{-3}&8.80 \cdot 10^{-6} & 3.23 \cdot 10^{-7}& 2.58 \cdot 10^{-8} & \cdots \\ \hline
		5& &3.43\cdot10^{-8}&6.13 \cdot 10^{-13} & 3.01 \cdot 10^{-16}& 8.46 \cdot 10^{-19} & \cdots\\ \hline
		\vdots& & \vdots & \vdots &\vdots &\vdots & \ddots
	\end{array}$
	\end{tabular}

\end{threeparttable}
\end{table}

%Consolidating all the best $\begin{matrix}\text{upper}\\\text{lower}\end{matrix}$ bounds:
\begin{table}[ht]
\centering
\begin{threeparttable}

	\caption{Best known bounds}
%	\caption{Best known bounds for $\underline{\delta}(Z_n,q)$}

	\begin{tabular}{c}
%	$\begin{array}{c|c|c|c|c|c}
%		&q=2&3&4&5&\cdots \\ \hline
%		n=2&.5&.333&.25&.2& \cdots \\ \hline
%		3&\substack{3.57\cdot 10^{-2} \\1.85\cdot 10^{-2}}  &\substack{1.84 \cdot 10^{-2} \\ 8.33\cdot 10^{-4} }& \substack{5.19 \cdot 10^{-3}\\ 5.31 \cdot 10^{-5} }& \substack{2.00 \cdot 10^{-3} \\ 3.22 \cdot 10^{-6}} & \cdots\\ \hline
%	
%		4&\substack{1.12\cdot10^{-3} \\ 1.11\cdot 10^{-12} }  &\substack{8.80 \cdot 10^{-6} \\ 6.64\cdot 10^{-392943} }& \substack{3.23 \cdot 10^{-7} \\ 9.42\cdot 10^{-233250395}
%	 }& \substack{2.58 \cdot 10^{-8} \\ - }& \cdots \\ \hline
%		5&\substack{3.43\cdot10^{-8} \\ - }  &\substack{6.13 \cdot 10^{-13} \\ - }& \substack{3.01 \cdot 10^{-16} \\ - }& \substack{8.46 \cdot 10^{-19} \\ - }& \cdots
%	\end{array}$
	$\begin{array}{c|c|c|c|c|c}
		\underline{\delta}(Z_n,q) &q=2&3&4&5&\cdots \\ \hline
		n=2 & 1/2 = .5 & 1/3 \approx .333 & 1/4 = .25 & 1/5 = .2 & \cdots \\ \hline
		3&\begin{matrix} .119 \\ 1/54 \approx 1.85\cdot 10^{-2}\end{matrix}  &\begin{matrix}1.84 \cdot 10^{-2} \\ 8.33\cdot 10^{-4} \end{matrix}& \begin{matrix}5.19 \cdot 10^{-3}\\ 5.31 \cdot 10^{-5} \end{matrix}& \begin{matrix}2.00 \cdot 10^{-3} \\ 3.22 \cdot 10^{-7} \end{matrix} & \cdots\\ \hline
	
		4&\begin{matrix}1.12\cdot10^{-3} \\ 1.11\cdot 10^{-12} \end{matrix}  &\begin{matrix}8.80 \cdot 10^{-6} \\ 6.64\cdot 10^{-392943} \end{matrix} & \begin{matrix}3.23 \cdot 10^{-7} \\ 9.42\cdot 10^{-233250395} \end{matrix} & \begin{matrix}2.58 \cdot 10^{-8} \\ - \end{matrix}& \cdots \\ \hline
		5&\begin{matrix}3.43\cdot10^{-8} \\ - \end{matrix} &\begin{matrix}6.13 \cdot 10^{-13} \\ - \end{matrix} & \begin{matrix}3.01 \cdot 10^{-16} \\ - \end{matrix} & \begin{matrix}8.46 \cdot 10^{-19} \\ - \end{matrix} & \cdots \\ \hline
		\vdots & \vdots & \vdots & \vdots & \vdots & \ddots
	\end{array}$
	\end{tabular}

	\begin{tablenotes}[flushleft]
		\item $n=2, q \geq 2$ from Theorem \ref{dZ2}.
		\item $n=3, q\geq 2$ Upper from Section \ref{prob}.
		\item $n=3, q\geq 2$ Lower from Corollary \ref{dZ3}.
		\item $n=3, q=2$ Lower conjectured to be 1/28 in Section \ref{DeB}.
		\item $n\geq 4, q\geq 2$ Upper from Section \ref{IV}.
		\item $n=4, q=2$ Lower from Theorem \ref{dZn}.
		\item $n=4, q\geq3$ Lower from Theorem \ref{dZn}.
	\end{tablenotes}

\end{threeparttable}
\end{table}
